# Supplementary material for: Careful About What App Promotion Ads Recommend! Detecting and Explaining Malware Promotion via App Promotion Graph
Source: arXiv:2410.07588 source file (2025-01-17)
Supplement: Supplementary file 1 [file 11-appendix.tex]

% \newpage
% \begin{appendices}
% \newpage
% \newpage
% \clearpage
% \footnote{\href{https://apk.apkdownqd6.top/}{Website of the malicious downloader}} 
%  \appendix


% \subsection{Descriptions and Links of PUAs/Malware with User Review}




% \begin{figure}[h!]
%     \centering
%     \includegraphics[width=\columnwidth]{figs/bad_chatgpt_review.png}
%     \caption{A user review for ``Ask AI - Chat with Chatbot" complaining about the subscription issue}
%     \label{fig:chatgpt_review}
% \end{figure}


% \subsection{Examples of App Promotion Ads}

% \begin{textblock*}{10cm}(1cm,12.5cm) % {block width} (coords)
%       \centering 
%   \begin{figure}[H]
%     \begin{subfigure}[]{0.25\linewidth}
%       \centering
%       \includegraphics[width=\linewidth]{figs/Banner (1).jpg}
%       \caption{Banner Ad}
%       \label{fig:banner}
%     \end{subfigure}
%     \begin{subfigure}[]{0.25\linewidth}
%       \centering
%       \includegraphics[width=\linewidth]{figs/rewarded (1).png}
%       \caption{Rewarded Ad}
%       \label{fig:rewarded}
%     \end{subfigure}

%     \vspace{0.001em}
%     \begin{subfigure}[]{0.25\linewidth}
%       \centering
%       \includegraphics[width=\linewidth]{figs/Appwall.jpg}
%       \caption{Appwall Ad}
%       \label{fig:more_apps}
%     \end{subfigure}
%     \begin{subfigure}[]{0.25\linewidth}
%       \centering
%       \includegraphics[width=\linewidth]{figs/Popup.jpg}
%       \caption{Interstitial Ad}
%       \label{fig:interstitial}
%     \end{subfigure}
%     \caption{Examples of app promotion ads}
%     \label{fig:ad_formats}
%   \end{figure}
% \end{textblock*}


% \begin{textblock*}{8cm}(11.3cm,2.2cm) % {block width} (coords)
% \subsection{Case Study and Mechanisms of Malware Promotion}
% \end{textblock*}

% \begin{textblock*}{9cm}(11cm,3.5cm) % {block width} (coords)
% \centering
%   \begin{figure}[H]
%     \centering
%     \begin{subfigure}[]{0.25\linewidth}
%       \centering
%       \includegraphics[width=\linewidth]{figs/Screenshot_magnet.jpg}
%       \caption{Trojan Dropper}
%       \label{fig:magnet_customized}
%     \end{subfigure}
%     \hspace{0.01\linewidth}
%     \begin{subfigure}[]{0.25\linewidth}
%       \centering
%       \includegraphics[width=\linewidth]{figs/android.view.View_2023.02.25-15.28.05_com.lomolsoft.dict.cedict (1).jpg}
%       \caption{Trojan}
%       \label{fig:lomol_appwall}
%     \end{subfigure}

%     % \vspace{0.01em}
%     \begin{subfigure}[]{0.25\linewidth}
%       \centering
%       \includegraphics[width=\linewidth]{figs/com.MommyLongsLegsPart2Guide.GuideMommyLongLetsPart2 (1).png}
%       \caption{Aggressive Adware}
%       \label{fig:wallpaper}
%     \end{subfigure}
%     \hspace{0.01\linewidth}
%     \begin{subfigure}[]{0.25\linewidth}
%       \centering
%       \includegraphics[width=\linewidth]{figs/Screenshot_rogue.jpg}
%       \caption{Rogue Security Software}
%       \label{fig:rogueSecurity}
%     \end{subfigure}
%     \caption{Case study on malware promotion}
%     \label{fig:case_malware}
%   \end{figure}
% \end{textblock*}

% \begin{textblock*}{9cm}(11.3cm,15.3cm) % {block width} (coords)
% \centering
%   \begin{figure}[H]
%     \centering
%     \begin{subfigure}[]{0.65\linewidth}
%       \centering
%       \includegraphics[width=\linewidth]{figs/Shared_code.pdf}
%       \caption{Examples of custom ad-based propagation}
%       \label{fig:channel_shared_codes}
%     \end{subfigure}
    
%     \vspace{0.01em}
    
%     \begin{subfigure}[]{0.65\linewidth}
%       \centering
%       \includegraphics[width=\linewidth]{figs/Ad_service.pdf}
%       \caption{Examples of ad library-based propagation}
%       \label{fig:channel_ad_lib}
%     \end{subfigure}
%     \caption{Examples of malware/PUA propagation mechanisms}
%     \label{fig:propagation_channels}
%   \end{figure}
% \end{textblock*}
